# Supplementary material for: WZ production cross-section measurement at 7 TeV and 8 TeV center of mass energies within the Compact Muon Solenoid experiment
Source: arXiv:1403.2978 source file (2014-03-12)
Supplement: Supplementary file 1 [file A01-SpacetimeAlgebra.tex]

\chapter{Spacetime algebra}\label{app:spacetimealgebra}

The \emph{geometric algebra} or \emph{Clifford algebra} is an algebraic system with increasing
interest in the physicist community due to the simplicity of its grammar and the geometric meaning
of vector multiplication, linking geometry to the physical interpretation of the 
world~\cite{2003Oerstedmedallect}. This language allows to re-express fundamental physics in a
vocabulary that is free from coordinates or indices, emphasizing the fundamental role of geometric
invariants in physics and clarifying the interpretation of many equations. In particular, the
interpretation of the Dirac matrices of the Dirac theory as the vectors of the basis of the 
ordinary spacetime~\cite{Hestenes03spacetimephysics} facilitates the comprehension of the 
geometric structure and physical interpretation of the Dirac theory. This formulation recovers the 
main results of the standard matrix version, whence simplifies the theory. This appendix will 
briefly introduce the geometric algebra topic in order to have an appetite-inducing effect in the
reader, but without enter in further or rigurous details. A comprehensive treatement may be found
in~\cite{d2003geometric}. 

\section{The geometric product}
Given a vector space $V$ over a $\mathbb{K}$ field, and a quadratic form $Q$ mapping the vector
space to the scalar field, $Q:\,V\to\mathbb{K}$; the operation between vectors of $V$, $a$, $b$ and
$c$, fulfilling the following properties:
\begin{enumerate}
	\item associative
		\begin{equation}
			a(bc) = (ab)c = abc
		\end{equation}
	\item distributive over addition
		\begin{equation}
			a(b+c)=ab+ac
		\end{equation}
	\item the square of any vector is a scalar, 
		\begin{equation}
			Q(a)=a^2\in\mathbb{K}
			\label{app1:eq:squarescalar}
		\end{equation}
\end{enumerate}
is defined as the \emph{geometric product}. Note that there are no commutative property and also 
the square of the vector is not necessarily positive. A first consequence is the existence of 
multiplicative inverse of any non-null vector $a^2\neq0$, 
\begin{equation*}
	a^{-1}=\frac{a}{a^2}
\end{equation*}
Note as $a^2$ is a scalar and therefore commute with any object, it is possible to use the 
fractional notation. This is not true in general due to the non-commutativity of the geometric 
product, $a^{-1}b\neq ba^{-1}$ in general, accordingly there is no sense in the expression 
$\frac{b}{a}$.

As the geometric product of two vectors is not commutative, it is possible to split the product of 
two vectors in its symetric and antisymetric parts,
\begin{equation}
	ab=a\cdot b+a\wedge b
\end{equation}
where the \emph{inner product} is defined as
\begin{equation}
	a\cdot b:= \frac{1}{2}\left(ab+ba\right)
\end{equation}
and the \emph{outer product} is
\begin{equation}
	a\wedge b:=\frac{1}{2}\left(ab-ba\right)
\end{equation}
Note that $a\cdot b=b\cdot a$ and $a\wedge b=-b\wedge a$.

Observing that, as $(a+b)\in V$ and by \eqref{app1:eq:squarescalar}, $(a+b)^2\in\mathbb{K}$
\begin{equation*}
	(a+b)^2 = (a+b)(a+b)=a^2+ab+ba+b^2 \in \mathbb{K}
\end{equation*}
Therefore, $ab+ba=(a+b)^2-a^2-b^2$ is also a scalar. The inner product is, then, regarded as the
standard scalar product between two vectors. 

\paragraph*{}
Note that the geometric product of two parallel vectors must commute, 
\begin{gather*}
	\text{if } a || b \Rightarrow b=\alpha a\;, \alpha\in\mathbb{K},\text{ then}\\
	ab=a(\alpha a)=\alpha aa=(\alpha a)a=ba,
\end{gather*}
which may be expressed as the equivalences,
\begin{equation*}
	a||b\Leftrightarrow 
	\begin{cases}
		ab=ba\\
		a\wedge b =0\\
		ab=a\cdot b
	\end{cases}
\end{equation*}
Conversely, the geometric product of two perpendicular vectors must anticommute,
\begin{gather*}
	\text{if } a \perp b \Rightarrow a\cdot b =0,\text{ then}\\
	0=a\cdot b=\frac{1}{2}(ab+ba)\Rightarrow ab=-ba
\end{gather*}
and, therefore, 
\begin{equation*}
	a\perp b\Leftrightarrow
	\begin{cases}
		ab=-ba\\
		a\cdot b =0\\
		ab=a\wedge b
	\end{cases}
\end{equation*}
Therefore, the geometric product provides a measure of the relative direction of the vectors.
Commutativity means collinear vectors, whence anticommutativity is establishing orthogonal
vectors.

The outer product defines a new object, called
\emph{bivector} or a 2-graded multivector, outside of the vector space $V$ of dimension $n$,
but forming a new vector space $V\wedge V$. And by successives applications of the outer 
product over n-independent, orthogonal vectors it is possible to build n-vector spaces, 
\begin{equation*}
	V\wedge\overbrace{\cdots}^k \wedge V\equiv\bigwedge^k V,
\end{equation*}
where the dimensions of each space is given by the possibility of
build $k$ combinations of the n-ortogonal vectors without repetition,~\ie 
\begin{equation*}
	dim\left(\bigwedge^kV\right)=\frac{n!}{k!(n-k)!}
\end{equation*}
In turn, those linear spaces form a graded linear space, the 
geometric algebra $\mathcal{G}$, the elements of which are called \emph{multivectors}. 
Assuming a basis set of $n$ independent, orthonormal vectors $\{e_i\}$ defines a basis
for the entire algebra $\mathcal{G}$ generated by these vectors.
\begin{center}
	\begin{tabular}{cccccc}
		$1$,  &  $\{e_i\}$, &  $\{e_i\wedge e_j\}$, & $\{e_i\wedge e_j\wedge e_k\}$, & $\dots$, &
				$e_1\wedge e_2\wedge\dots e_n\equiv I$\\
		scalars,& vectors, &  bivectors, &  trivectors, & \dots, & pseudoescalar 
	\end{tabular}
\end{center}
These objects constitute the basis of the $2^n$ linear space of the geometric algebra.
Any multivector that is built as the outer product of r independent vectors is called a 
\emph{blade} and denoted as $A_r$, a blade is also called a multivector of grade $r$. Each 
multivector of the geometric algebra can be decomposed in sum of r-grades through the 
grade-projection operator, $\langle\; \rangle_r$ which outputs the grade-r portion of the 
multivector:
\begin{equation*}
	M = \sum_{r=0}^n\langle M\rangle_r
\end{equation*}

The highest-grade blade in the algebra, the $n$-grade $I$, is called the \emph{pseudoscalar} or 
\emph{directed volume element}. The pseudoscalar contains all the information of the vector space 
$V$ over which the algebra is built, and also defines the duality operations for the algebra:
the multiplication of a $r$-grade multivector by $I$ results in a $(n-r)$-grade multivector.
As the dual of a 0-grade or scalar is the $n$-grade $I$ called the pseudoscalar, consequently the 
dual of a vector is a $(n-1)$-grade, called \emph{pseudovectors}; and so on.

\section{Planea}
The algebra of the 2-dimensional space may be generated with a set of orthonormal vectors in 
$\mathbb{R}$, \[ \{e_1,e_2\} \] such that
\begin{equation*}
	\begin{aligned}
		& e_{1}e_{2}=e_{1}\wedge e_{2}\\
		& e_1^2=e_2^2=1
	\end{aligned}
\end{equation*}
The algebra $\mathcal{G}_2$ is generated with the basis
\begin{center}
	\begin{tabular}{lcccr}
		$\{$ & $1$,  &  $e_1,e_2$, &  $e_1e_2$ & $\}$\\
		     & scalar,& vectors, &  bivector, & 
	\end{tabular}
\end{center}
forming a linear space of $2^2=1+2+1=4$ elements. Note as $e_i$ are ortogonals, $e_ie_j=-e_je_i$,
therefore the bivector or pseudoscalar $e_1e_2\equiv I$, 
\begin{equation*}
	I^2=(e_1e_2)(e_1e_2)=-(e_1e_2)(e_2e_1)=-e_1e_2^2e_1= -e_1^2=-1
\end{equation*}
Note that the pseudoscalar $I$ is defining the directed area element of the plane defined by
the vectors $e_1$ and $e_2$ chosen as right-handed oriented. In addition, applying the pseudoscalar
to $e_1$,
\begin{align*}
	Ie_1&=(e_1e_2)e_1=-e_2\\
	e_1I&=e_1(e_1e_2)=e_2
\end{align*}
and to $e_2$
\begin{align*}
	Ie_2&=(e_1e_2)e_2=e_1\\
	e_2I&=e_2(e_1e_2)=-e_1
\end{align*}
Therefore, the pseudoscalar $I$ \emph{rotates} the vector $e_1$ to $e_2$ and $e_2$ to $e_1$. Thus,
$I$ has two complementary geometric interpretations as unique oriented area in the plane and an
oriented right angle rotation in the plane. The rotation operator may be extended using the 
geometric product of two unit vectors $a=a_1e_1+a_2e_2$ ($a^2=0$) and 
$b=b_1e_1+b_2e_2$ ($b^2=1$), being the length of the directed arc 
in the unit circle between the two vectors the angle $\theta$. Then,
\begin{align*}
	a\cdot b &= cos\theta\\
	a\wedge b&= sin\theta(e_1\wedge e_2)=sin\theta(e_1e_2)=Isin\theta
\end{align*}
Thus, the geometric product of two vectors defines a new entity called \emph{rotor}, $U_{\theta}=ab$
which belongs to the even subalgebra $\mathcal{G}^+$. Note the name of rotor is justified by the 
fact that the multiplication of any vector by the rotor, it will rotate the vector in the $I$-plane
through an angle $\theta$.

In fact, two vectors
The pseudoscalar can be used 
and commute with any vector and multivector,
\begin{equation*}
	(e_1e_2e_3)e_k = -e_1e_2e_ke_3=e_1e_ke_2e_3=-e_ke_1e_2e_3
\end{equation*}
